# Supplementary material for: Local Rule-Based Explanations of Black Box Decision Systems
Source: arXiv:1805.10820 source file (2018-05-28)
Supplement: Supplementary file 1 [file appendix.tex]

%\HIDE{
\newpage
\appendix

\section{Additional Experiments}

This section includes some further experimental results.

\begin{table}[t]
\setlength{\tabcolsep}{0.7mm}
\small
\begin{tabular}{c|c|c|c|c|c|c}
\toprule
\textit{Distance} & $\mathit{hit}$ & $\mathit{fidelity}$ & $\mathit{l{\text -}fidelity}$ & $|c|$ & $|p|$ & $\mathit{nf}$ \\
\midrule
cosine   & $.938 {\pm} .24$ & $\mathbf{.976 {\pm} .11}$ & $.936 {\pm} .24$ & $4.4 {\pm} 2.5$ & $\mathbf{2.1 {\pm} 1.8}$ & $1.9 {\pm} 1.0$ \\
minmax & $.958 {\pm} .19$ & $.965 {\pm} .15$ & $.956 {\pm} .17$ & $4.5 {\pm} 2.7$ & $2.3 {\pm} 2.3$ & $\mathbf{1.8 {\pm} 0.9}$ \\
neuclid  & $\mathbf{.966 {\pm} .17}$ & $.967 {\pm} .15$ & $.\mathbf{963 {\pm} .19}$ & $\mathbf{4.3 {\pm} 2.6}$ & $2.2 {\pm} 2.1$ & $1.8 {\pm} 1.0$ \\
\bottomrule
\end{tabular}
\caption{Comparison of distance measures on the \emph{german} dataset.}
\label{tab:dist_comp}
%\vspace{-8mm}
\end{table}

\subsection{Comparing Distance Functions}

A key element of the neighborhood generation is the distance function used by the genetic algorithm. A legitimate question is whether the results of the approach are affected by the choice of the distance. For instance, \cite{wachter2017counterfactual} reports considerable differences in their output of counterfactual instance based on the choice of the distance in their stochastic optimization approach.
Table \ref{tab:dist_comp} reports basic measures contrasting the \textit{normalized Euclidean} distance adopted by \textbf{LORE} with 
 \textit{cosine} and \textit{min-max} distance. The table does not highlight any considerable difference. This can be justified by the fact that, following instance generation, there are phases, such as decision tree building, that abstracts instances to patterns, resulting in resilience against variability due to the distance function adopted.

\subsection{Coverage of Global Features}

%{\color{red} S: ho cercato di riformulare questa sezione, ma con calma ne riparliamo.}

In this section we replicate the experiment in \cite{ribeiro2016should} to measure the \textit{faithfulness} of explanations with respect to classifiers that are interpretable by design, i.e., decision tree (\textbf{DT}) and logistic regression with L2 regularization (\textbf{LR}).
However, differently from \cite{ribeiro2016should} we do not have to specify a fixed number of ``gold'' features, i.e., the most important features that can be used by the global model. 
To make a proper comparison, we rank the features by importance values returned by DT and LR. 
Then, we consider an increasing number of gold features going from the top-2 to the top-10, and use them in \textbf{LORE}.
In our experiments, we study both recall over the black box, as in the global method of \cite{ribeiro2016should}, and the precision. %In fact, in the evaluation of a local approach, it is very relevant to measure the ability of the local classifier to capture features which are globally important, but not necessarily all of them. While high recall means that the quality of a local classifier depends on the fact that it is considering locally the same set of attributes which are globally important. However, in case a local predictor use all global important features this means that the local one is not capturing more than the global one. 

Figure~\ref{fig:global_coverage} reports the results of these analysis at the variation of the number of features included in data, for the \textit{german} (first and second row) and \textit{compass} (third and last row) datasets.
Since LIME requires the number of gold features for the explanation, we run two versions of it: LIME which uses as number of features the same number of the gold features (from 2 to 10), and LIME--4 which uses 4 as number of features, corresponding to the average length of the premises of LIME.
%It is interesting to notice some aspects.
LIME, which is based on logistic regression, %as local interpretable classifier 
has a better performance with LR compared to DT.
On the other hand \textbf{LORE}, which is based on decision trees, has better performance with DT compared to LR.
Contrasting \textbf{LORE} and LIME, the former has better performance in terms of precision (due to its local nature), while the latter has better recall if 6 or more gold features are provided by the user (due to its global nature).
\textbf{LORE} overcomes LIME in identifying the minimum set of gold features that should characterize an explanation, while LIME is better than \textbf{LORE} in recalling in an explanation the global features used by the black box when a considerable number of gold features is considered (and suggested to LIME).
%However, this could also be not a strong point.

\begin{figure}[t]
    \centering
    \hspace{-2mm}
    	\includegraphics[trim = 2mm 0mm 1mm 0mm, clip,width=0.49\linewidth]{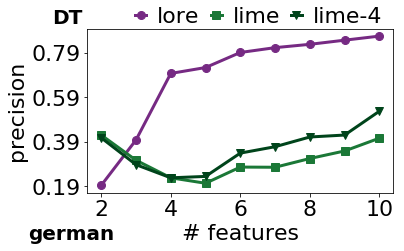}\vspace{-6.3mm}
   		\includegraphics[trim = 2mm 0mm 1mm 0mm, clip,width=0.49\linewidth]{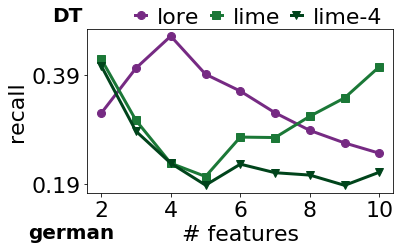}
        \includegraphics[trim = 2mm 0mm 1mm 0mm, clip,width=0.49\linewidth]{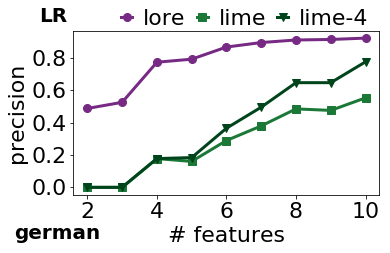}
   		\includegraphics[trim = 2mm 0mm 1mm 0mm, clip,width=0.49\linewidth]{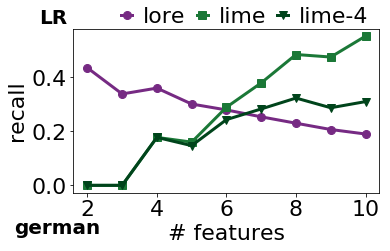} 
        \includegraphics[trim = 2mm 0mm 1mm 0mm, clip,width=0.49\linewidth]{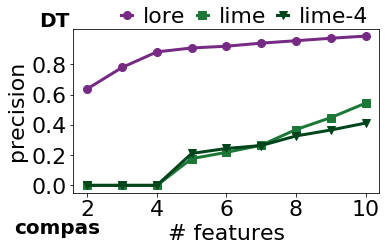} \vspace{-6.3mm}
   		\includegraphics[trim = 2mm 0mm 1mm 0mm, clip,width=0.49\linewidth]{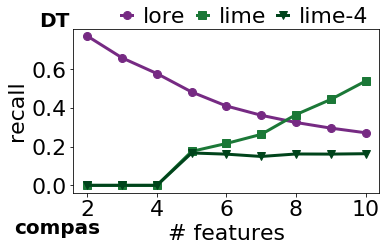}
        \includegraphics[trim = 2mm 0mm 1mm 0mm, clip,width=0.49\linewidth]{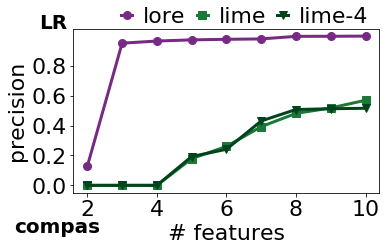}
   		\includegraphics[trim = 2mm 0mm 1mm 0mm, clip,width=0.49\linewidth]{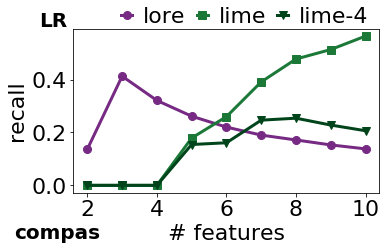}   
 	\vspace{-3mm}
\caption{Precision and recall at the variation of the number of features.}
\label{fig:global_coverage}
\vspace{-1mm}
\end{figure}

\subsubsection{Rules vs Stochastic Counterfactuals}

Regarding the counterfactual part of local explanations, we now compare \textbf{LORE} with 
the stochastic optimization approach  of \cite{wachter2017counterfactual}. It looks for an instance $x'$ as close as possible to a given $x$, but for which the black box outputs a different prediction. The Manhattan distance weighted by the inverse median absolute deviation is used in the search of $x'$. The approach returns $x'$ as result. As already observed in the related work section, \textbf{LORE} is more general, since it provides one or more counterfactual rules, which generalize patterns of instances such as $x'$, hence providing the user with more informative output. In some sense, the stochastic optimization approach is limited to the phase of neighborhood generation, i.e., it looks for an element in $Z_{\neq}$. 
{\color{blue}In order to make a fair comparison with our approach, we have implemented the stochastic optimization as an alternative fitness function of the genetic neighborhood generation. Questa frase e' sbagliata, correggiamola insieme.}
{\color{red} S: ancora non capisco bene questo ...}
Let us call \texttt{opt} our overall approach with such a change.
Table~\ref{tab:counterfactual_comp} shows the performances of the two methods on  $\mathit{nf}$  (number of falsified conditions in counterfactual rules),  $\mathit{c\text{-}hit}$ (rate of agreement of black box and counterfactual decision for counterfactual instance), and  $\mathit{cl{\text -}fidelity}$ (f1-measure of agreement of black box and counterfactual decision for instances covered by the counterfactual rule). The first is a measure of complexity of counterfactual explanations: \textbf{LORE} returns shorter explanations than \texttt{opt}. The last two are measures of fidelity on the neighborhood instances that satisfy the premise of the counterfactual rules. They are considerably higher for \textbf{LORE}, especially for the \texttt{german} dataset.
Once again, the merit is in the ability of \textbf{LORE} to generate a neighborhood that covers a dense and compact area around the instance under analysis. As a consequence, changes suggested by the counterfactuals tend to be small, and decision trees built from the neighborhood are not large.

\begin{table}[t]
\begin{tabular}{ccccc}
\toprule
\textit{Dataset} & \textit{Method} &  $\mathit{nf}$ &  $\mathit{c\text{-}hit}$ &  $\mathit{cl{\text -}fidelity}$ \\
\midrule
{\multirow{2}{*}{german}} & lore & \textbf{1.52 $\pm$ 1.18} & \textbf{.7765 $\pm$ .38} & \textbf{.5355 $\pm$ .43} \\
 						  & opt & 14.80 $\pm$ 1.59 & .3118 $\pm$ .47 & .2297 $\pm$ .36 \\
 \hline
{\multirow{2}{*}{compas}} & lore & \textbf{1.84 $\pm$ 0.78} & \textbf{.8694 $\pm$ .37} & \textbf{.8611 $\pm$ .41} \\
 						  & opt & 6.24 $\pm$ 1.45 & .8036 $\pm$ .38 & .7555 $\pm$ .34 \\
\bottomrule
\end{tabular}
\caption{\textbf{LORE} vs OPT: performance of counterfactual rules.}
\label{tab:counterfactual_comp}
\vspace{-3mm}
\end{table}

% esperimento rimuovibile non aggiunge nulla di importante al paper
%\paragraph{Robustness to Artificial Features}
%\begin{figure}[t]
%    \centering
%    \hspace{-2mm}
%    	\includegraphics[trim = 2mm 0mm 1mm 0mm, clip,width=0.49\linewidth]{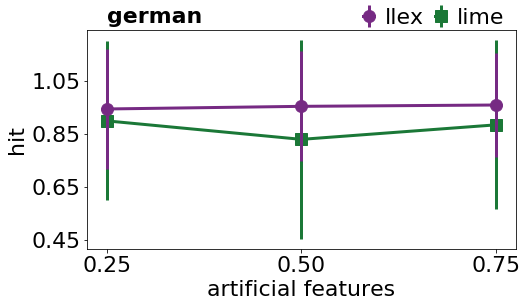} 
%   		\includegraphics[trim = 2mm 0mm 1mm 0mm, clip,width=0.49\linewidth]{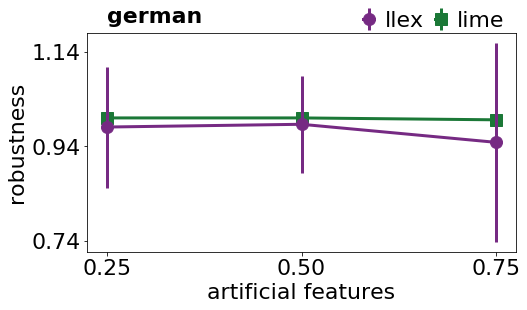} 
%        \includegraphics[trim = 2mm 0mm 1mm 0mm, clip,width=0.49\linewidth]{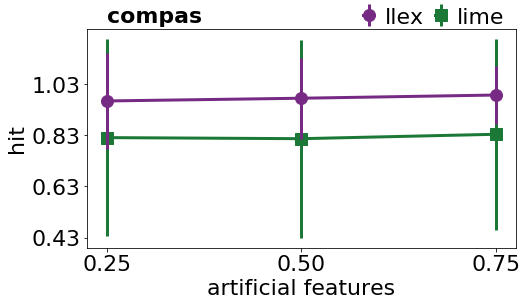} 
%   		\includegraphics[trim = 2mm 0mm 1mm 0mm, clip,width=0.49\linewidth]{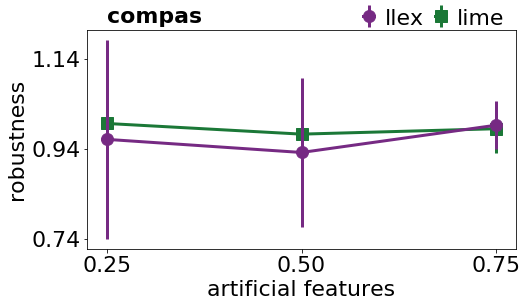} 
% 	\vspace{-5mm}
%\caption{TODO.}
%\label{fig:robustness}
%%\vspace{-3mm}
%\end{figure}

%}
